# Supplementary material for: Temporal Graphs and Temporal Network Characteristics for Bio-Inspired Networks During Optimization
Source: arXiv:2110.00506 source file (2021-10-01)
Supplement: Supplementary file 1 [file appendix.tex]

\appendix

\section{Appendixes}

To start the appendixes, use the \verb+\appendix+ command.
This signals that all following section commands refer to appendixes
instead of regular sections. Therefore, the \verb+\appendix+ command
should be used only once---to setup the section commands to act as
appendixes. Thereafter normal section commands are used. The heading
for a section can be left empty. For example,
\begin{verbatim}
\appendix
\section{}
\end{verbatim}
will produce an appendix heading that says ``APPENDIX A'' and
\begin{verbatim}
\appendix
\section{Background}
\end{verbatim}
will produce an appendix heading that says ``APPENDIX A: BACKGROUND''
(note that the colon is set automatically).

If there is only one appendix, then the letter ``A'' should not
appear. This is suppressed by using the star version of the appendix
command (\verb+\appendix*+ in the place of \verb+\appendix+).

\section{A little more on appendixes}

Observe that this appendix was started by using
\begin{verbatim}
\section{A little more on appendixes}
\end{verbatim}

Note the equation number in an appendix:
\begin{equation}
E=mc^2.
\end{equation}

\subsection{\label{app:subsec}A subsection in an appendix}

You can use a subsection or subsubsection in an appendix. Note the
numbering: we are now in Appendix~\ref{app:subsec}.

Note the equation numbers in this appendix, produced with the
subequations environment:
\begin{subequations}
\begin{eqnarray}
E&=&mc, \label{appa}
\\
E&=&mc^2, \label{appb}
\\
E&\agt& mc^3. \label{appc}
\end{eqnarray}
\end{subequations}
They turn out to be Eqs.~(\ref{appa}), (\ref{appb}), and (\ref{appc}).
